# Supplementary material for: Aligning Language Models with Preferences through f-divergence Minimization
Source: arXiv:2302.08215 source file (2023-06-06)
Supplement: Supplementary file 1 [file previous.appendices.formal.tex]

\section{TMP-formal: temporary placeholder for displaced material}

\subsection{TMP-formal-table}
\begin{table*}
\begin{centering}
\begin{tabular}{ccccc}
\toprule
$D_f(\pit||p)$ & {\footnotesize{}$f$} & {\footnotesize{}$f'$} & {\footnotesize{}$f^{'}\left(\frac{\pi_{\theta}(x)}{p(x)}\right)$}& {\footnotesize{}$f^{'}(\infty)$}\tabularnewline
\midrule
{\footnotesize{}forward KL} & {\footnotesize{}$f(t)=-\log t$} & {\footnotesize{}$f^{'}(t)=-\frac{1}{t}$} & {\footnotesize{}$-\frac{p(x)}{\pi_{\theta}(x)}$}& {\footnotesize{}$0$}\tabularnewline
% \hline 
{\footnotesize{}reverse KL} & {\footnotesize{}$f(t)=t\log t$} & {\footnotesize{}$f^{'}(t)=\log t+1$} & {\footnotesize{}$-\left(\log\frac{p(x)}{\pi_{\theta}(x)}\right)+1$}& {\footnotesize{}$\infty$}\tabularnewline
% \hline 
Total variation & {\footnotesize{}$f(t)=|1-t|$} & {\footnotesize{}$f^{'}(t)=\begin{cases}
1 & \text{for }t>1\\
-1 & \text{for }t<1
% \\\text{undefined} & \text{for }t=1
\end{cases}$} & {\footnotesize{}$\begin{cases}
1 & \text{for }\frac{\pi_{\theta}(x)}{p(x)}>1\\
-1 & \text{for }\frac{\pi_{\theta}(x)}{p(x)}<1
% \\\text{undefined} & \text{for }\pi_{\theta}(x)=p(x)
\end{cases}$}& {\footnotesize{}$1$}\tabularnewline
% \hline 
{\footnotesize{}Jensen-Shannon} & {\footnotesize{}$f(t)=t\log\frac{2t}{t+1}+\log\frac{2}{t+1}$} & {\footnotesize{}$f^{'}(t)=\log\frac{2t}{t+1}$} & {\footnotesize{}$\log 2-\log\left(1+\frac{p(x)}{\pi_{\theta}(x)}\right)$}& {\footnotesize{}$\log 2$}\tabularnewline
% \hline 
{\footnotesize{}Squared Hellinger distance} & {\footnotesize{}$f(t)=(1-\sqrt{t})^{2}$} & {\footnotesize{}$f^{'}(t)=1-\frac{1}{\sqrt{t}}$} & {\footnotesize{}$1-\sqrt{\frac{p(x)}{\pi_{\theta}(x)}}$}& {\footnotesize{}$1$}\tabularnewline
% \hline 
{\footnotesize{}Chi-squared divergence} & {\footnotesize{}$f(t)=(t-1)^{2}$} & {\footnotesize{}$f^{'}(t)=2(t-1)$} & {\footnotesize{}$2\left(\frac{\pi_{\theta}(x)}{p(x)}-1\right)$}& {\footnotesize{}$\infty$}\tabularnewline
% \hline 
{\footnotesize{}Le Cam distance} & {\footnotesize{}$f(t)=\frac{1-t}{2t+2}$} & {\footnotesize{}$f^{'}(t)=-\frac{1}{(1+t)^{2}}$} & {\footnotesize{}$-\left(\frac{p(x)}{p(x)+\pi_{\theta}(x)}\right)^{2}$}& {\footnotesize{}$0$}\tabularnewline
\bottomrule
\end{tabular}
\par\end{centering}
\caption{Some common $f$-divergences $D_f(\pi_\theta||p)$. 
%Note that forward KL divergence and reverse KL divergence  $D_f(p||\pi_\theta)$ instead of $D_f(\pi_\theta||p)$.
In the convention of this table, the $f$ shown corresponds to the order of arguments $D_f(\pit||p)$. Thus the forward KL between the target $p(x)$ and the model, $\text{KL}(p||\pit)$, corresponds to $D_{-\!\log t} (\pit||p)$, and similarly for the reverse KL, $\text{KL}(\pit||p)$, which corresponds to $D_{t \log t} (\pit||p)$, etc. Note that for symmetric divergences (TV and JS) the order of arguments is indifferent\ptmdI{: $\text{TV}(\pit||p)=\text{TV}(p||\pit)$, $\text{JS}(\pit||p)=\text{JS}(p||\pit)$.}
\label{tab:f-dpg-loss-appendix}}
\end{table*}

\subsection{TMP-formal-simplified-theorem}

\begin{thm*}[Theorem 1 repeated]
\label{thm:f-dpg-appendix}
Let $p$ and $\pit$ be distributions over a discrete set $\mathcal{X}$ such that  at least one of the following  conditions holds: 
(i) $\forall \theta \in \Theta, \Supp(p)\subset \Supp(\pit)$, or 
(ii) $\Supp(\pit)$ does not depend on $\theta$. Then:
% \ptmdI{$Supp(\pit)$ does not change with $\theta$,}
% $Supp(p) \subset Supp(\pit)$, 
% then:\fmdI{(13/01/2023) Note the change in the condition. I think this is more general, but can be discussed.}
%\fmdI{We should say somewhere something about $f'(\pit(x)/0$) in this equation.}
\begin{align}
    \nabla_{\theta}D_{f}(\pi_{\theta}||p)=E_{x\sim\pi_{\theta}}\left[f^{'}\left(\frac{\pi_{\theta}(x)}{p(x)}\right)\nabla_{\theta}\log\pi_{\theta}(x)\right].
\label{Eq.:fdpg-gradient-appendix}
\end{align}
\end{thm*}
\ptmdI{The full proof of this theorem is provided in Appendix  \ref{app:proofs}, but let's already give a sketch, under the more restrictive assumption that $Supp(\pit)=Supp(p
) = S$.}
Based on Eq. \eqref{Eq.:f-divergence-simplified} we then have:\fmdI{(08/01/2023) This takes a lot of space. Should we delegate the whole proof (including the special case) to the Appendix?}
\fdyI{Hmm, I think that the straight forward proof for the special case is kind of attractive point that we have. For me, I would look for another section to save the space}
 % $D_{f}(\pi_{\theta}||p)=\sum_{\forall x}p(x)f\left(\frac{\pi_{\theta}(x)}{p(x)}\right).$
\begin{align*}
\nabt D_{f}(\pit||p) &= \nabt\ \ \E_{x\sim p}\ f(\frac{\pit(x)}{p(x)})\\
& =\nabt \sum_{x\in S}p(x)f\left(\frac{\pit(x)}{p(x)}\right)\\
 % & =\sum_{x\in S}p(x)\nabt f\left(\frac{\pit(x)}{p(x)}\right)\\
 & =\sum_{x\in S}p(x)f^{'}\left(\frac{\pit(x)}{p(x)}\right)\nabt \frac{\pit(x)}{p(x)}\\
 & =\sum_{x\in S}f^{'}\left(\frac{\pit(x)}{p(x)}\right)\nabt \ \pit(x)\\
 & =\sum_{x\in S}\pit(x)f^{'}\left(\frac{\pit(x)}{p(x)}\right)\nabt\log\pit(x)\\
 &= E_{x\sim\pit}\left[f^{'}\left(\frac{\pit(x)}{p(x)}\right)\nabt \log\pit(x)\right],
\end{align*}
where the third line involves an application of the chain-rule for the multidimensional variable $\theta$.

% \begin{proof}
% See Appendix \ref{app:proofs}
% \end{proof}
% In third equation we used chain rule, and the term $\nabla_{\theta}\frac{\pi_{\theta}(x)}{p(x)}$ makes the expectation with respect to $p(x)$ canceled out. The last equation we used log derivative trick, so that this can be approximated with samples from $\pi_{\theta}$. 

% \fmdI{(06/01/2023) I stopped my updating here, will continue later.}







\newpage
 
\section{$f$-divergences: equivalent definitions}\label{app:generalized_divergence}
Here we give a general definition of f-divergences between two probability distributions, without restrictions on the supports, in a useful ``symmetrical'' format, following \cite{liese2006divergences}. We then show that this definition is equivalent with the definition of Eq.~\ref{Eq.:f-divergence} \cite{polyanski},
\fmdI{(11/01/2023) I do not see this proof yet, will add it!}
\fdyI{I meant the general f-divergence can be simplfied to Eq. \ref{Eq.:f-divergence-simplified} (not Eq.~\ref{Eq.:f-divergence}) of which proof was intended in  Eq. ~\ref{Eq.:f-divergence-simplified2}}
and then
give examples of common $f$-divergences in the notation of the general definition.
\begin{definition*}[$f$-divergence: ``symmetrical'' format]
The $f$-divergence between two probability distributions $p$ and
$q$ over a discrete set $\mathcal{X}$ can be defined as
\begin{align}
D_{f}(p||q)\doteq \sum_{\{x:\ p(x)>0,\ q(x)>0\}}q(x)\ f(\frac{p(x)}{q(x)}) \quad +f(0)\ q(p=0) \quad +f^{*}(0)\ p(q=0)
\label{eq:generalized_divergence}
\end{align}


where the generator function $f:\ptmdI{(0,\infty)}\rightarrow\mathbb{R}$%
\fmdI{(11/01/2023) We need to use the open interval $(0,\infty)$ because $f$ need not be  defined in $0$ (e.g. $-\log t$), although it can be extended to $0$ with some care.}
is a convex function satisfying $f(1)=0$.
We denote by $q(p=0)$
the $q$-mass of the set $\{x:p(x)=0\}$, i.e. $q(p=0)=\sum_{\{x:p(x)=0\}}q(x)$
and similarly for $p(q=0)$.  
\end{definition*}
In this definition, the function $f^{*}(t)$ is the so-called \emph{perspective transform} of $f$
defined by $f^{*}(t)=t\ f(\frac{1}{t})$. It can be shown to also be a convex function
$f^{*}:\ptmdI{(0,\infty)} \rightarrow\mathbb{R}$ with $f^{*}(1)=0$ and
$f^{**}=f$. Also, $f(0) \in (0,\infty]$ can be defined as the (always existing) limit $f(0)\doteq \lim_{t\rightarrow 0} f(t)$, and similarly $f^{*}(0) \in (0,\infty]$ as $f^{*}(0)\doteq \lim_{t\rightarrow 0} f^{*}(t) = \lim_{t\rightarrow 0}\ t\ f(1/t)$ \cite{hiriart2013convex}. 



\ptmdI{HHHHH Here now (11/01/2023) HHHHH}






We now define the convention following \citet{liese2006divergences, polyanski}: 
\begin{itemize}
\item $f(0)=\lim_{t\rightarrow0}f(t)$, $f^{*}(0)=\lim_{t\rightarrow0}tf(\frac{1}{t})$
\item $0f(\frac{a}{0})=\lim_{t\rightarrow0}tf(\frac{a}{t})=af^{*}(0)$ for
$a>0$
\item $0f(0)=0,\ 0f^{*}(0)=0$, including the case where $f(0)=\infty$
\item $0f(\frac{0}{0})=0$
\end{itemize}
While it is not necessary for Theorem \ref{thm:f-dpg}, we show that, using the definition defined above, the general $f$-divergence without the assumption on the support can be simplified as follows.\label{Eq.:f-divergence-simplified2}
\begin{align*}
D_{f}(p||q) & =\sum_{\{x:p(x)>0,\ q(x)>0\}}q(x)f(\frac{p(x)}{q(x)})+f(0)q(p=0)+f^{*}(0)p(q=0)\\
 & =\sum_{\{x:p(x)q(x)>0\}}q(x)f(\frac{p(x)}{q(x)})+\sum_{\{x:p(x)=0,q(x)>0\}}q(x)f(0)+\sum_{\{x:p(x)>0,q(x)=0\}}q(x)f^{*}(0)+\sum_{\{x:p(x)=0,q(x)=0\}}0\\
 & =\sum_{\{x:p(x)q(x)>0\}}q(x)f(\frac{p(x)}{q(x)})+\sum_{\{x:p(x)=0,q(x)>0\}}q(x)f(\frac{p(x)}{q(x)})+\\ &\quad \sum_{\{x:p(x)>0,q(x)=0\}}q(x)f(\frac{p(x)}{q(x)})+\sum_{\{x:p(x)=0,q(x)=0\}}q(x)f(\frac{p(x)}{q(x)})\\
 & =\sum_{\forall x}q(x)f(\frac{p(x)}{q(x)})
\end{align*}


We now see how the generalized definition of $f$-divergence can be
adopted to the common divergences. 

\paragraph*{Forward, reverse KL}

\[
\text{KL}(p||q)=D_{f}(p||q)=D_{f^{*}}(q||p)
\]
 where $f(t)=t\log t$ with $f(0)=0,$$f^{*}(t)=-\log t$ with $f^{*}(0)=\infty$.
We can write $\text{KL}(p||q)$ with the generalized $f$-divergence;
\begin{align*}
\text{KL}(p||q) & =\sum_{\{x:p(x)>0,\ q(x)>0\}}q(x)f(\frac{p(x)}{q(x)})+f(0)q(p=0)+f^{*}(0)p(q=0)\\
 & =\sum_{\{x:p(x)>0,\ q(x)>0\}}q(x)\frac{p(x)}{q(x)}\log\frac{p(x)}{q(x)}+0+\infty p(q=0)\\
 & =\begin{cases}
\sum_{\{x:p(x)>0\}}p(x)\log\frac{p(x)}{q(x)} & \text{if }p(q=0)>0\\
\infty & \text{o.w.}
\end{cases}\\
 & =\begin{cases}
E_{x\sim p}\left[\log\frac{p(x)}{q(x)}\right] & \text{if }p(q=0)>0\\
\infty & \text{o.w.}
\end{cases}
\end{align*}
 

Similarly we have $\text{KL}(q||p)=\infty$ with $f(t)=t\log t$, we get 
\[
KL(q||p)=\begin{cases}
E_{x\sim q}\left[\log\frac{q(x)}{p(x)}\right] & \text{if }q(p=0)>0\\
\infty & \text{o.w.}
\end{cases}
\]


\paragraph*{Total variation divergence}

For Total variation divergence, 
\[
TV(p||q)=D_{f}(p||q)=D_{f^{*}}(q||p)=TV(q||p)
\]
with $f(t)=\frac{1}{2}|1-t|$ with $f(0)=\frac{1}{2}$ and $f^{*}(t)=f(t)$,
and $f^{*}(0)=\frac{1}{2}$. We can write $TV(p||q)$ with the generalized
$f$-divergence as follows
\begin{align*}
TV(p||q) & =\sum_{\{x:p(x)>0,\ q(x)>0\}}q(x)f(\frac{p(x)}{q(x)})+f(0)q(p=0)+f^{*}(0)p(q=0)\\
 & =\frac{1}{2}\sum_{\{x:p(x)>0,\ q(x)>0\}}q(x)\left|1-\frac{p(x)}{q(x)}\right|+\frac{1}{2}q(p=0)+\frac{1}{2}p(q=0)
\end{align*}
For example, in the extreme case where $\text{Supp}(p)\cap\text{Supp}(p)=\emptyset$,
we get the first term null, and second and third term equal to 0.5,
implying that $TV(p||q)=1$.
\section{Proofs and definitions}\label{app:proofs}

\begin{proof}[proof of Theorem \ref{thm:f-dpg}]
Note that without the restriction on the support of $p(x)$,
\[
D_{f}(\pi_{\theta}||p)=\sum_{\{x:\pi_{\theta}(x)p(x)>0\}}p(x)f(\frac{\pi_{\theta}(x)}{p(x)})+f(0)p(\pi_{\theta}=0)+f^{*}(0)\pi_{\theta}(p=0)
\]
therefore, 
\begin{align*}
\nabla_{\theta}D_{f}(\pi_{\theta}||p) & =\sum_{\{x:\pi_{\theta}(x)p(x)>0\}}p(x)\nabla_{\theta}f(\frac{\pi_{\theta}(x)}{p(x)})+f^{*}(0)\nabla_{\theta}\pi_{\theta}(p=0)+f(0)\nabla_{\theta}p(\pi_{\theta}=0)\\
 & =\sum_{\{x:\pi_{\theta}(x)p(x)>0\}}p(x)f^{'}(\frac{\pi_{\theta}(x)}{p(x)})\nabla_{\theta}\frac{\pi_{\theta}(x)}{p(x)}+f^{*}(0)\nabla_{\theta}\pi_{\theta}(p=0)+f(0)\nabla_{\theta}p(\pi_{\theta}=0)\\
 & =\sum_{\{x:\pi_{\theta}(x)p(x)>0\}}\pi_{\theta}(x)f^{'}(\frac{\pi_{\theta}(x)}{p(x)})\nabla_{\theta}\log\pi_{\theta}(x)+f^{*}(0)\nabla_{\theta}\pi_{\theta}(p=0)+f(0)\nabla_{\theta}p(\pi_{\theta}=0)\\
 & =\sum_{\{x:\pi_{\theta}(x)p(x)>0\}}\pi_{\theta}(x)f^{'}(\frac{\pi_{\theta}(x)}{p(x)})\nabla_{\theta}\log\pi_{\theta}(x)+f^{*}(0)\nabla_{\theta}\sum_{\{x:p(x)=0,\pi_{\theta}(x)>0\}}\pi_{\theta}(x)\\
 &\quad +f(0)\nabla_{\theta}p(\pi_{\theta}=0),\ \text{by definition of }\pi_{\theta}(p=0)\\
 & =\sum_{\{x:\pi_{\theta}(x)p(x)>0\}}\pi_{\theta}(x)f^{'}(\frac{\pi_{\theta}(x)}{p(x)})\nabla_{\theta}\log\pi_{\theta}(x)+\sum_{\{x:p(x)=0,\pi_{\theta}(x)>0\}}\pi_{\theta}(x)f^{*}(0)\nabla_{\theta}\log\pi_{\theta}(x)\\
 &\quad +f(0)\nabla_{\theta}p(\pi_{\theta}=0)\\
 & =\sum_{\{x:\pi_{\theta}(x)p(x)>0\}}\pi_{\theta}(x)f^{'}(\frac{\pi_{\theta}(x)}{p(x)})\nabla_{\theta}\log\pi_{\theta}(x)+\sum_{\{x:p(x)=0,\pi_{\theta}(x)>0\}}\pi_{\theta}(x)f^{'}(\infty)\nabla_{\theta}\log\pi_{\theta}(x)\\
 &\quad +f(0)\nabla_{\theta}p(\pi_{\theta}=0),\ \because f^{*}(0)=f^{'}(\infty)\\
 & =\sum_{\{x:\pi_{\theta}(x)>0\}}\pi_{\theta}(x)f^{'}(\frac{\pi_{\theta}(x)}{p(x)})\nabla_{\theta}\log\pi_{\theta}(x)+f(0)\nabla_{\theta}p(\pi_{\theta}=0)
\end{align*}

The condition (i) stating that the support of $p$ is contained in the support of $\pi_{\theta}$ for all $\theta \in \Theta$ implies that $\nabla_{\theta}p(\pi_{\theta}=0)=\nabla_{\theta}0=0$, and the condition (ii) that the support of $\pi_{\theta}$ does not depend on $\theta$ further implies that $\nabla_{\theta}p(\pi_{\theta}=0)=0$, which concludes the proof.
% The condition (i) $\forall \theta \in \Theta, \Supp(p)\subset \Supp(\pit)$ implies that $\nabla_{\theta}p(\pi_{\theta}=0)=\nabla_{\theta}0=0$, and 
% (ii) $\Supp(\pit)$ does not depend on $\theta$ further implies $\nabla_{\theta}p(\pi_{\theta}=0)=0$, which
% concludes the proof.
\end{proof}

Especially, in the context of LMs, $\pi_{\theta}$ is typically a standard softmax-based autoregressive model which has full support over $\mathcal{X}$, meaning that $Supp(\pi_{\theta}) = \mathcal{X}$ and ${x:\pi_{\theta}(x)=0}=\emptyset$, thus satisfying condition (i).
% it is clear for all $x\in\mathcal{X}$, there
% exist $\delta>0\ \text{such that }\pi_{\theta}(x)>\delta$. 


Note that we use the notation $f^{'}(\infty)\doteq f^{*}(0)$ which is employed by \cite{polyanski} and is motivated by the fact that $\lim_{t\rightarrow\infty}f^{'}(t)=\lim_{t\rightarrow\infty}\frac{1}{t}f(t)=f^{*}(0)$ (See \citep{hiriart2013convex}). This notation allows to write $f^{'}(\frac{\pi_{\theta}(x)}{p(x)})$ instead of $f^{\ast}(0)$ when
$p(x)=0$ and $\pi_{\theta}(x)>0$ and therefore to simplify the writing
of $\nabla_{\theta}D_{f}(\pi_{\theta},p)$.

\begin{thm*}[Theorem \ref{thm:f-dpg} with $D_f(p||\pit)$]
Let $p$ and $\pit$ be distributions over a discrete set $\mathcal{X}$ such that at least one of the following  conditions holds: 
(i) $\forall \theta \in \Theta, \Supp(p)\subset \Supp(\pit)$, or 
(ii) $\Supp(\pit)$ does not depend on $\theta$.
Then:
\[
\nabla_{\theta}D_{f}(p||\pi_{\theta})=E_{x\sim\pi_{\theta}}\left[f^{*'}(\frac{\pi_{\theta}(x)}{p(x)})\nabla_{\theta}\log\pi_{\theta}(x)\right]
\]
\end{thm*}

\begin{proof}
Note that without the restriction on the support of $p(x),$
\begin{align*}
D_{f}(p||\pi_{\theta}) & =\sum_{\{x:\pi_{\theta}(x)p(x)>0\}}\pi_{\theta}(x)f(\frac{p(x)}{\pi_{\theta}(x)})+f(0)\pi_{\theta}(p=0)+f^{*}(0)p(\pi_{\theta}=0)\\
 & =\sum_{\{x:\pi_{\theta}(x)p(x)\ge0\}}\pi_{\theta}(x)f(\frac{p(x)}{\pi_{\theta}(x)})+f^{*}(0)p(\pi_{\theta}=0)
\end{align*}
with $f(0)=f(\frac{p(x)}{\pi_{\theta}(x)})$ for $\{x:\pi_{\theta}(x)>0,p(x)=0\}$
and $f(0)\pi_{\theta}(p=0)=\sum_{\{x:\pi_{\theta}(x)>0,p(x)=0\}}\pi_{\theta}(x)f(\frac{p(x)}{\pi_{\theta}(x)})$.
Therefore, 
\begin{align*}
\nabla_{\theta}D_{f}(p||\pi_{\theta}) & =\sum_{\{x:\pi_{\theta}(x)>0,p(x)\ge0\}}\nabla_{\theta}\pi_{\theta}(x)f(\frac{p(x)}{\pi_{\theta}(x)})+\sum_{\{x:\pi_{\theta}(x)p(x)\ge0\}}\pi_{\theta}(x)f^{'}(\frac{p(x)}{\pi_{\theta}(x)})(-\frac{p(x)}{\pi_{\theta}(x)^{2}})\nabla_{\theta}\pi_{\theta}(x)\\&\qquad+f^{'}(\infty)\nabla_{\theta}p(\pi_{\theta}=0)\\
 & =\sum_{\{x:\pi_{\theta}(x)>0,p(x)\ge0\}}\nabla_{\theta}\pi_{\theta}(x)\left[f(\frac{p(x)}{\pi_{\theta}(x)})-f^{'}(\frac{p(x)}{\pi_{\theta}(x)})(\frac{p(x)}{\pi_{\theta}(x)})\right]+f{}^{'}(\infty)\nabla_{\theta}p(\pi_{\theta}=0)\\
 & =\sum_{\{x:\pi_{\theta}(x)>0,p(x)\ge0\}}\nabla_{\theta}\pi_{\theta}(x)\left[\frac{p(x)}{\pi_{\theta}(x)}f^{*}(\frac{\pi_{\theta}(x)}{p(x)})-\left(f^{*}(\frac{\pi_{\theta}(x)}{p(x)})-\frac{\pi_{\theta}(x)}{p(x)}f^{*'}(\frac{\pi_{\theta}(x)}{p(x)})\right)(\frac{p(x)}{\pi_{\theta}(x)})\right]\\&\quad+f^{'}(\infty)\nabla_{\theta}p(\pi_{\theta}=0)\\
 & =\sum_{\{x:\pi_{\theta}(x)>0,p(x)\ge0\}}\nabla_{\theta}\pi_{\theta}(x)f^{*'}(\frac{\pi_{\theta}(x)}{p(x)})+f^{'}(\infty)\nabla_{\theta}p(\pi_{\theta}=0)\\
 & =\sum_{\{x:\pi_{\theta}(x)>0,p(x)\ge0\}}\pi_{\theta}(x)f^{*'}(\frac{\pi_{\theta}(x)}{p(x)})\nabla_{\theta}\log\pi_{\theta}(x)+\nabla_{\theta}\sum_{\{x:\pi_{\theta}(x)=0,p(x)>0\}}f^{'}(\infty)p(x)
\end{align*}
For the third equation we use the definition of perspective function
$f(t)=tf^{*}(\frac{1}{t})$ and its derivative, $f^{'}(t)=f^{*}(\frac{1}{t})+tf^{*'}(\frac{1}{t})(-\frac{1}{t^{2}})=f^{*}(\frac{1}{t})-\frac{1}{t}f^{*'}(\frac{1}{t})$.
For the last step, as aforementioned, with either condition (i) stating that the support of $p$ is contained in the support of $\pi_{\theta}$ for all $\theta \in \Theta$, or (ii) that the support of $\pi_{\theta}$ does not depend on $\theta$, the last term goes to zero, thus completing the proof.
\end{proof}

\begin{thm*}[Baseline based on $f$-divergence property]
For $f$-divergence $D_{f}(\pi_{\theta}||p)$ with any generator $f$,
there exists a generator $g$ with the same divergence $D_{f}(\pi_{\theta}||p)=D_{g}(\pi_{\theta}||p)$ such that
\begin{align*}
\nabla_{\theta}D_{g}(\pi_{\theta}||p) & =E_{x\sim\pi_{\theta}}\left[\left(f^{'}\left(\frac{\pi_{\theta}(x)}{p(x)}\right)-b\right)\nabla_{\theta}\log\pi_{\theta}(x)\right]\\
 & =\nabla_{\theta}D_{f}(\pi_{\theta}||p)
\end{align*}
\end{thm*}

\begin{proof}
Recall that %the facts of $f$-divergence that 
$D_{f}(\pi_{\theta}||p)=D_{g}(\pi_{\theta}||p)$
%if and only if exists $b\in\mathbb{R}$ such that 
\ptmdI{when}
$g(x)=f(x)-b(x-1)$, for $b\in\mathbb{R}$ %,$ with arbitrary $b\in\mathbb{R}$.
Therefore, $\nabla_{\theta}D_{f}(\pi_{\theta}||p)=\nabla_{\theta}D_{g}(\pi_{\theta}||p)$
with $g^{'}\left(\frac{\pi_\theta(x)}{p(x)}\right)=f^{'}\left(\frac{\pi_\theta(x)}{p(x)}\right)-b$ 
% Recall the facts of $f$-divergence that $D_{f}=D_{g}$ if and only
% if $g(x)=f(x)-b(x-1),$ with arbitrary $b\in\mathbb{R}$.
% {\footnotesize{}\begin{align*}
% \nabla_{\theta}D_{g}(\pi_{\theta},p) & =E_{x\sim\pi_{\theta}}\left[g^{'}\left(\frac{\pi_{\theta}(x)}{p(x)}\right)\nabla_{\theta}\log\pi_{\theta}(x)\right]\\
%  & =E_{x\sim\pi_{\theta}}\left[\left(f^{'}\left(\frac{\pi_{\theta}(x)}{p(x)}\right)-b\right)\nabla_{\theta}\log\pi_{\theta}(x)\right]\\
%  & =E_{x\sim\pi_{\theta}}\left[f^{'}\left(\frac{\pi_{\theta}(x)}{p(x)}\right)\nabla_{\theta}\log\pi_{\theta}(x)\right]\\& \quad -bE_{x\sim\pi_{\theta}}\left[\nabla_{\theta}\log\pi_{\theta}(x)\right]\\
%  % & =E_{x\sim\pi_{\theta}}\left[f^{'}\left(\frac{\pi_{\theta}(x)}{p(x)}\right)\nabla_{\theta}\log\pi_{\theta}(x)\right]\\&\quad -b\sum_{\forall x}\left[\nabla_{\theta}\pi_{\theta}(x)\right]\\
%  & =E_{x\sim\pi_{\theta}}\left[\left(f^{'}\left(\frac{\pi_{\theta}(x)}{p(x)}\right)\right)\nabla_{\theta}\log\pi_{\theta}(x)\right]\\
%  & =\nabla_{\theta}D_{f}(\pi_{\theta},p)
% \end{align*}}
\end{proof}



\begin{algorithm}[tb]
   \caption{$f$-DPG}
   \label{alg:f_dgp}
\begin{algorithmic}
   \STATE {\bfseries Input:}  unnormalized target distribution $P(\cdot)$, initial model $a(\cdot)$, $D_f$ generator $f(\cdot)$
   % \FOR{$i=1$ {\bfseries to} $m-1$}
   \STATE {\bfseries Initialize:} $\pit(\cdot) \gets a(\cdot)$, $Z \gets 0$, $N \gets 0$
   \FOR{each iteration do}
   \FOR{each episode do}
   \STATE sample $x$ from $\pit(\cdot)$
   \STATE $N \gets N+1$
   %\STATE $Z \gets Z+\frac{P(x)/\pit(x)-Z}{N}$
   \STATE $Z \gets Z+\frac{(P(x)/\pit(x))-Z}{N}$
   \qquad \COMMENT{Estimate $Z$ with historical samples}
   \STATE $p(\cdot) \gets P(\cdot)/Z$
   \STATE $\theta \gets \theta + \alpha^{(\theta)}f^{'}\left(\frac{\pit(x)}{p(x)}\right)\nabt\log\pit$
   \ENDFOR
   \ENDFOR
   \STATE {\bfseries Output:}  $\pit$
\end{algorithmic}
\end{algorithm}
